# Supplementary material for: Spectral Analysis of Diffusion Models with Application to Schedule Design
Source: arXiv:2502.00180 source file (2025-12-09)
Supplement: Supplementary file 1 [file Appendix_Estimating_a_circulant_matrix.tex]

\section{Estimating a circulant matrix}\label{sec:appendix_Circulant_from_toplitz}

Given a symmetric Toeplitz matrix B we aim to estimate a circulant matrix A that balances closely approximating the original matrix while preserving circulant properties.  Since both symmetric Toeplitz and circulant matrices are fully characterized by their first rows, the optimization is formulated in terms of ${\left\{ {X_{A}[k]} \right\}_{k=0}^{n-1}}$ and ${\left\{ {X_{B}[k]} \right\}_{k=0}^{n-1}}$, which represent the first rows of A and B, respectively:
$$\arg\min_{\left\{ {X_{A}[k]} \right\}_{k=0}^{n-1}} \left(X_{A}[k]-X_{B}[k]\right)^2\left(n-k\right)+ \left(X_{A}[k]-X_{B}[N-k]\right)^2\left(k\right)
$$
By differentiating the objective with respect to each element of ${X_{A}[k]}_{k=0}^{n-1}$ and setting the result equal to zero, we obtain:
$${X_{A}[k]} = \frac{X_{B}[k]\left(n-k\right)+X_{B}[n-k]k}{\left(n-k \right) + k} , \quad \text{for } k = 0, \dots, d-1$$
This approach leverages the structural properties of both matrices, ensuring that the estimated circulant matrix A remains as close as possible to B while preserving a circulant nature.
